# Supplementary material for: Structure Preserving Model Reduction of Parametric Hamiltonian Systems
Source: arXiv:1703.08345 source file (2017-03-24)
Supplement: Supplementary file 1 [file appendix.tex]

\section{Symplectic QR (SQR) decomposition} \label{chap:Append:1}

Similar to the QR decomposition for constructing an orthogonal matrix, for any full rank matrix $M$ of size $2n\times 2n$ we may have a decomposition
\begin{equation}
	M = AR,
\end{equation}
where $A$ is a symplectic square matrix (and not necessarily orthogonal) and $R$ has the structure
\begin{equation}
	R =
	\begin{pmatrix}
		S & T \\
		U & V
	\end{pmatrix}
\end{equation}
where $S$, $T$, $U$ and $V$ are all upper triangular square matrices of size $n$. Also $T$ and $U$ have zeros along the diagonal. The algorithm for a SQR is shown in Algorithm \ref{alg:Append:1}.

\begin{algorithm} 
\caption{Symplectic QR decomposition (SQR)} \label{alg:Append:1}
{\bf Input:} Full rank matrix $M = [u_1,\dots , u_k,v_1,\dots,v_k]$ of size $2n \times 2k$.
\begin{enumerate}
\item $\alpha \leftarrow \Omega(u_1,v_1)$
\item $e_1 \leftarrow \text{sign}(\alpha)\cdot u_1 / \sqrt{|\alpha|} $
\item $f_1 \leftarrow v_1 / \sqrt{|\alpha|}$
\item \textbf{for} $i\leftarrow 2$ \textbf{to} $k$
\item \hspace{0.5cm} $q \leftarrow u_i$
\item \hspace{0.5cm} $p \leftarrow v_i$
\item \hspace{0.5cm} \textbf{for} $j\leftarrow1$ \textbf{to} $i-1$
\item \hspace{0.5cm} \hspace{0.5cm} $q \leftarrow q - \Omega(q,f_j)e_j + \Omega(q,e_j)f_j$
\item \hspace{0.5cm} \hspace{0.5cm} $p \leftarrow p - \Omega(p,f_j)e_j + \Omega(p,e_j)f_j$
\item \hspace{0.5cm} \textbf{end for}
\item \hspace{0.5cm} $\alpha \leftarrow \Omega(q,p)$
\item \hspace{0.5cm} $e_i \leftarrow \text{sign}(\alpha) \cdot q / \sqrt{|\alpha|} $
\item \hspace{0.5cm} $f_i \leftarrow p / \sqrt{|\alpha|}$
\item \textbf{end for}
\item $A \leftarrow [e_1, \dots , e_k , f_1, \dots , f_k]$
\item $R \leftarrow A^+M$
\end{enumerate}

\vspace{0.5cm}
{\bf Output:} Matrix decomposition $M = AR$.
\end{algorithm}
